# Supplementary material for: A Search-based Neural Model for Biomedical Nested and Overlapping Event Detection
Source: arXiv:1910.10281 source file (2019-10-25)
Supplement: Supplementary file 1 [file appendix.tex]

%
% File emnlp2019.tex
%
%% Based on the style files for ACL 2019, which were
%% Based on the style files for EMNLP 2018, which were
%% Based on the style files for ACL 2018, which were
%% Based on the style files for ACL-2015, with some improvements
%%  taken from the NAACL-2016 style
%% Based on the style files for ACL-2014, which were, in turn,
%% based on ACL-2013, ACL-2012, ACL-2011, ACL-2010, ACL-IJCNLP-2009,
%% EACL-2009, IJCNLP-2008...
%% Based on the style files for EACL 2006 by 
%%e.agirre@ehu.es or Sergi.Balari@uab.es
%% and that of ACL 08 by Joakim Nivre and Noah Smith

\documentclass[11pt,a4paper]{article}
\usepackage[hyperref]{emnlp-ijcnlp-2019}
\usepackage{times}
\usepackage{latexsym}
\usepackage{graphicx}

\usepackage{url}

% table formatting
\usepackage{booktabs}
\usepackage{multirow}
\usepackage{makecell}

\usepackage{cleveref}
\crefformat{section}{\S#2#1#3} % see manual of cleveref, section 8.2.1
\crefformat{subsection}{\S#2#1#3}
\crefformat{subsubsection}{\S#2#1#3}

%\aclfinalcopy % Uncomment this line for the final submission

%\setlength\titlebox{5cm}
% You can expand the titlebox if you need extra space
% to show all the authors. Please do not make the titlebox
% smaller than 5cm (the original size); we will check this
% in the camera-ready version and ask you to change it back.

\title{Supplementary Materials for the Paper ``A Search-based Neural Model for Biomedical Nested and Overlapping Event Detection''}

\author{First Author \\
  Affiliation / Address line 1 \\
  Affiliation / Address line 2 \\
  Affiliation / Address line 3 \\
  \texttt{email@domain} \\\And
  Second Author \\
  Affiliation / Address line 1 \\
  Affiliation / Address line 2 \\
  Affiliation / Address line 3 \\
  \texttt{email@domain} \\}

\date{}

\begin{document}
\maketitle
\appendix

\section{Model Parameters}
\label{params}
% We implemented our model using the Chainer library.  We initialised the word embeddings using pre-trained embeddings while other embeddings are initialised using the normal distribution. All the embeddings and weight parameters were updated with mini-batch using the AMSGrad optimiser. We also incorporated early stopping to choose the number of training epochs and tuned hyper-parameters (dropout, learning rate and weight decay rate) using grid search. Table \ref{tab:1} shows the hyper-parameters used in our experiments.
\begin{table}[th!]
  \centering
  \resizebox{\linewidth}{!}{%
  \begin{tabular}{lr}
  \toprule[0.5pt]
  Parameter & Value/Dimension \\
  \midrule[0.5pt]
%   \textit{Common Parameters} &\\
%   \midrule[0.5pt]
  Mini-Batch Size &100 \\
  Word Embedding & 200 \\
  BiLSTM Word Embedding &100 \\
  Role Type Embedding & 10 \\
  Trigger/Argument Type Embedding & 20\\
  Early Stopping Patience & 5 \\
  Dropout & 0.5 \\
  Learning Rate & 0.001\\
    Hidden Layer Size & 60 \\
    Event Embedding &100  \\
%   \midrule[0.5pt]
%   \textit{Baseline Model}&\\
%   \midrule[0.5pt]
%   I/O Embedding & 2\\
%   Event Prediction Threshold &0.5  \\
%   Weight Decay Rate & 0 \\
%   \midrule[0.5pt]
%   \textit{Search-based Model}&\\
%   \midrule[0.5pt]
    Action Score Threshold &0.5  \\
    Beam Size & 8 \\
  Action Embedding & 4\\
  Weight Decay Rate & 0.001 \\
    \bottomrule[0.5pt]
  \end{tabular}
  }
 \caption{Hyper-parameters used in our experiments.}
 \label{tab:1}
\end{table}

% \bibliography{emnlp-ijcnlp-2019}
% \bibliographystyle{acl_natbib}

\end{document}
